# Supplementary material for: Factorized Inverse Path Tracing for Efficient and Accurate Material-Lighting Estimation
Source: arXiv:2304.05669 source file (2023-08-23)
Supplement: Supplementary file 1 [file camera_trajectory.tex]

\begin{figure}
    \centering
    \includegraphics[width=0.95\linewidth]{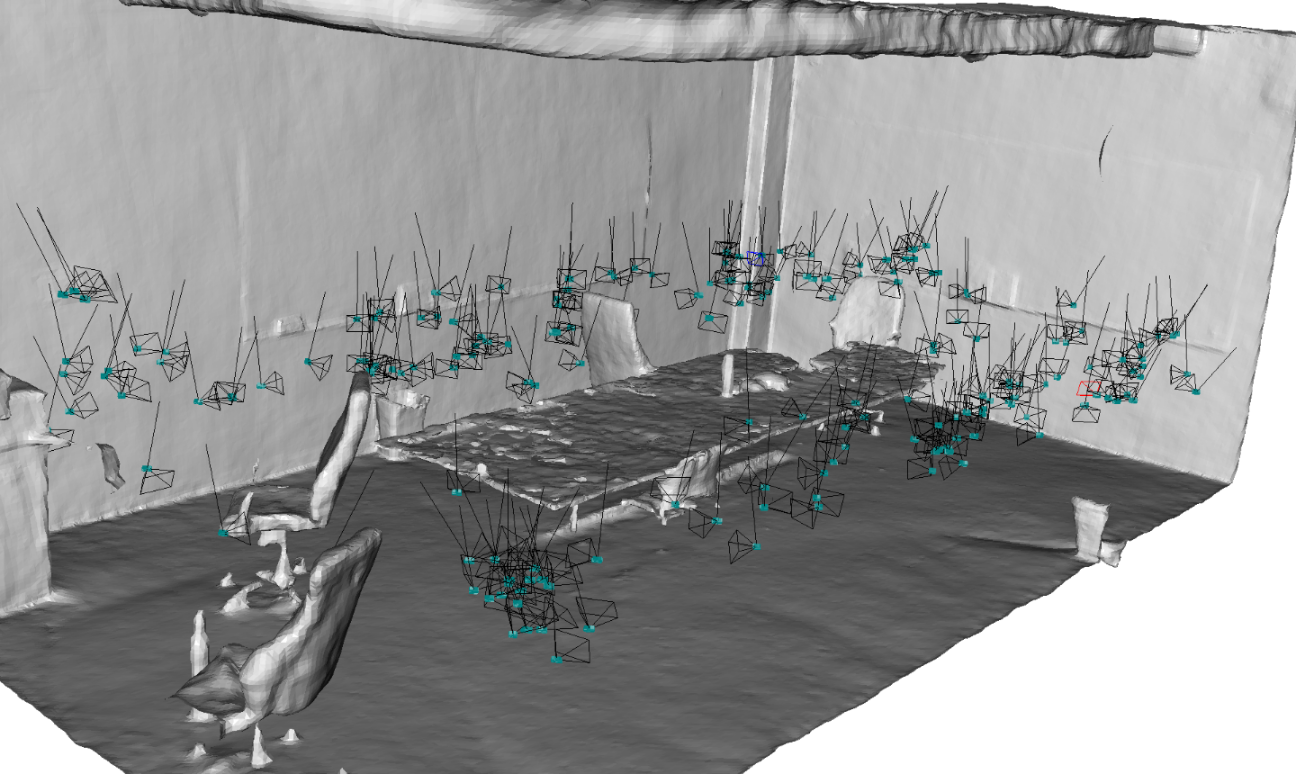}
    \includegraphics[width=0.95\linewidth]{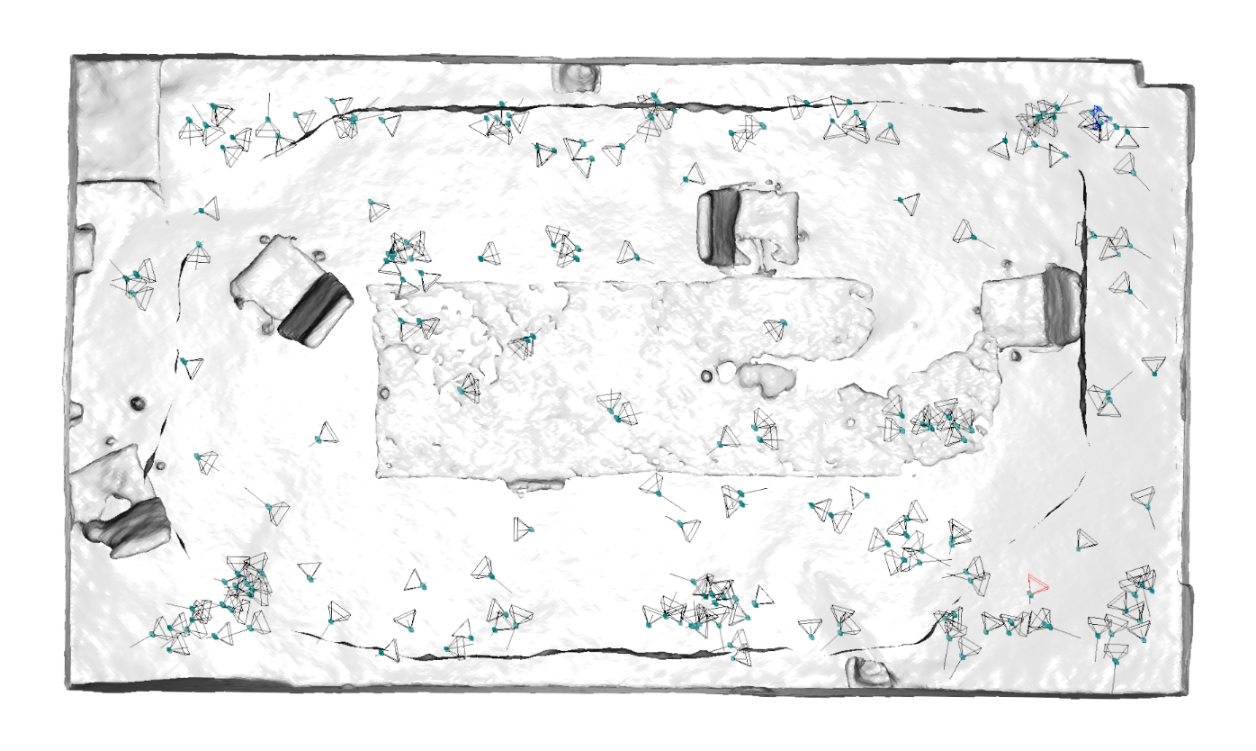}
    \includegraphics[width=0.95\linewidth]{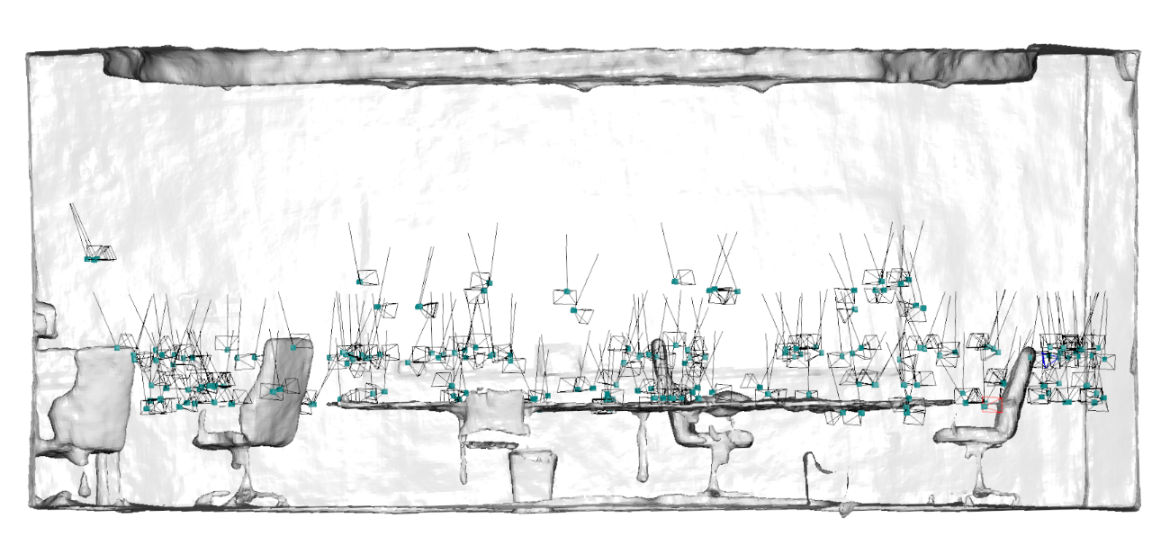}
    \caption{\textbf{Illustration of camera trajectory} for the Conference Room scene, shown in three views, together with estimated scene geometry from MonoSDF. Each camera is shown as small frustum, with up direction shown as vector in black.}
    \label{fig:camera_trajectory}
\end{figure}
