# Supplementary material for: Factorized Inverse Path Tracing for Efficient and Accurate Material-Lighting Estimation
Source: arXiv:2304.05669 source file (2023-08-23)
Supplement: Supplementary file 2 [file demo_lieccv22_relight.tex]

\begin{figure}
    \centering
    \includegraphics[width=0.95\linewidth]{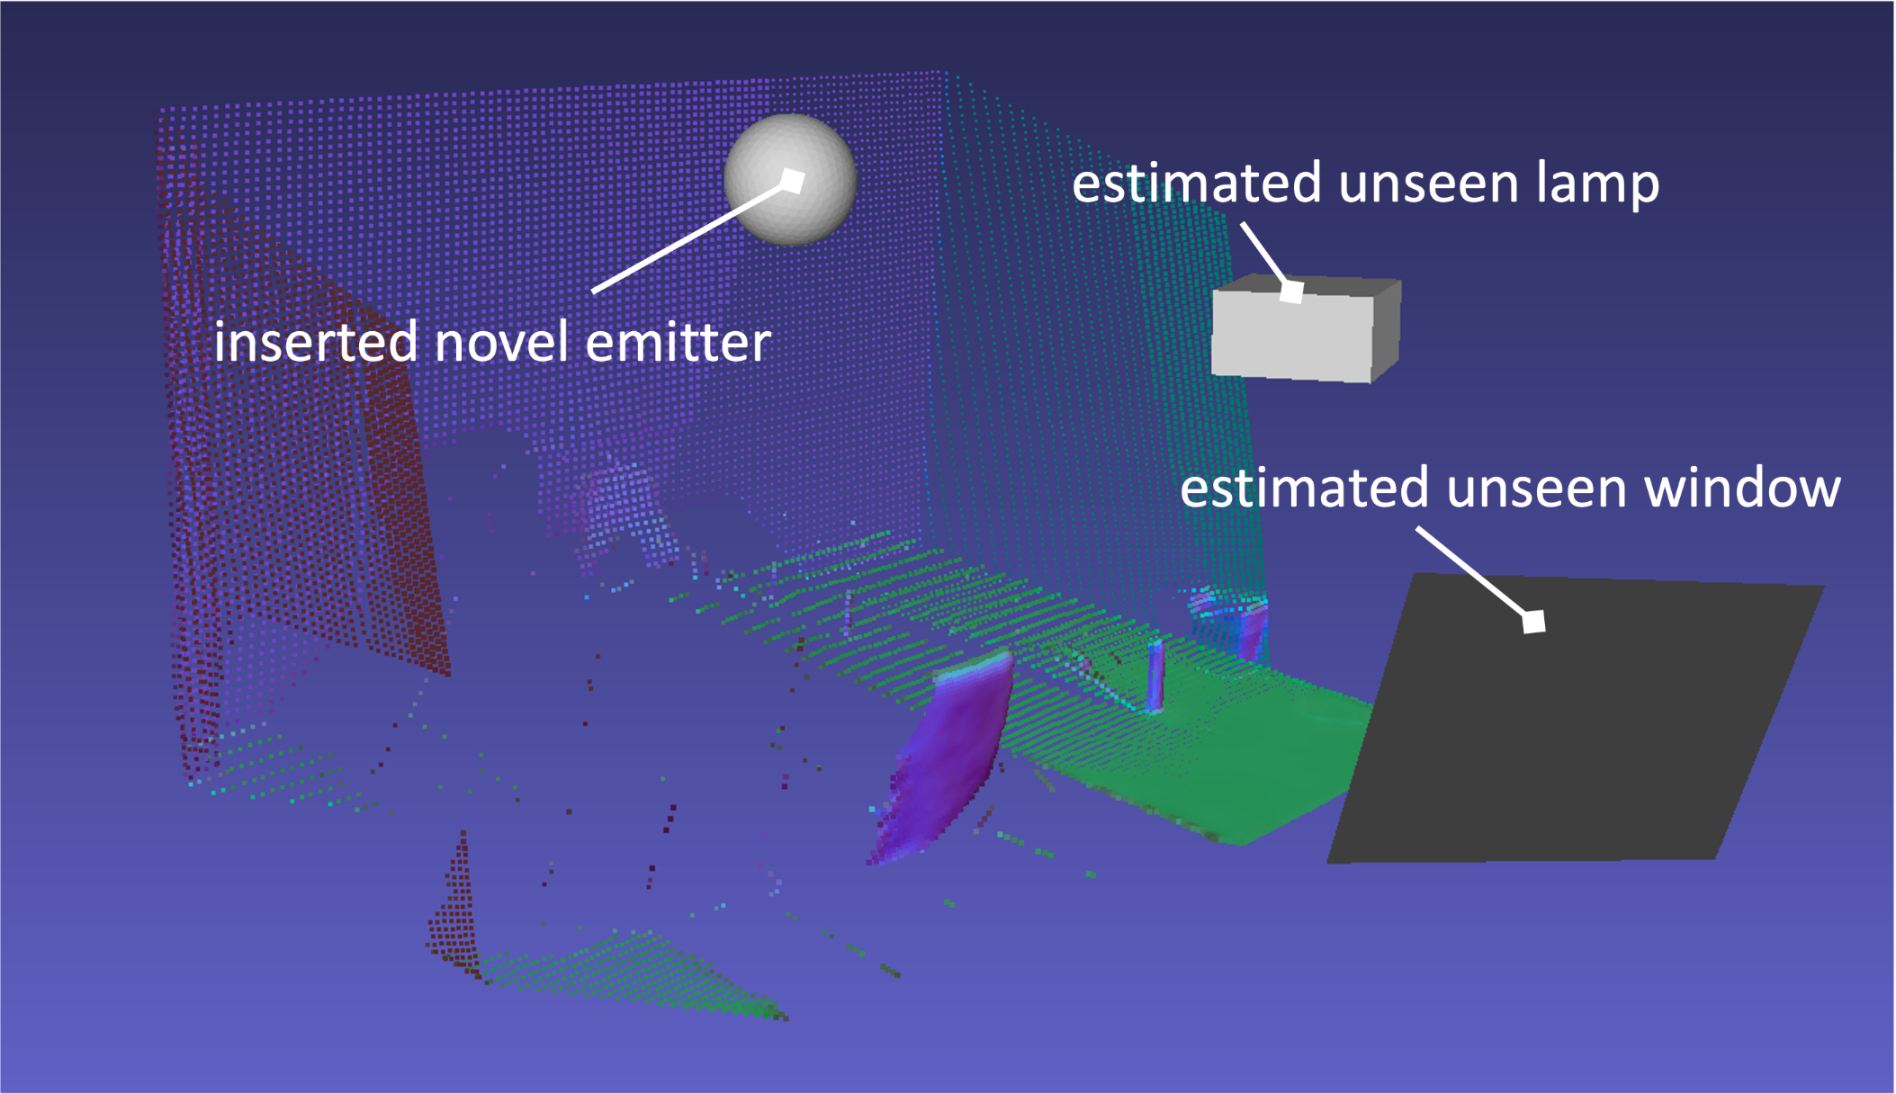}
    \caption{
    \textbf{Geometry, estimated and inserted emitters by \lieccv}, of the Conference room scene.}
    \label{fig:demo_lieccv22_relighting}
\end{figure}
